# Supplementary material for: Phonon-induced band gap renormalization by dielectric dependent global hybrid density functional tight-binding
Source: arXiv:2403.14210 ancillary file (2024-03-21)
Supplement: Supplementary file 1 [file supplmat.pdf]

# Supplementary Material:
# Phonon-induced band gap renormalization by dielectric dependent global hybrid density functional tight-binding

Tammo van der Heide,[1] Ben Hourahine,[2] Bálint Aradi,[1]
Thomas Frauenheim,[3,4] and Thomas A. Niehaus[5,*]

[1]*Bremen Center for Computational Materials Science, University of Bremen, 28359 Bremen, Germany*

[2]*SUPA, Department of Physics, The University of Strathclyde, Glasgow, G4 0NG, United Kingdom*

[3]*Constructor University, School of Science, Campus Ring 1, Bremen, Germany*

[4]*Institute for Advanced Study, Chengdu University, Chengdu 610106, China*

[5]*Univ Lyon, Université Claude Bernard Lyon 1, CNRS, Institut Lumière Matière, F-69622 Villeurbanne, France*

(Dated: March 20, 2024)

* thomas.niehaus@univ-lyon1.fr

## S1. SUPPLEMENTARY TABLES

| Temperature [K] | $a^{\text{C-dia}}$ [Å] | $a^{\text{Si-dia}}$ [Å] |
|---|---|---|
| 0 | 3.5616 | 5.4593 |
| 10 | 3.5620 | 5.4596 |
| 20 | 3.5623 | 5.4597 |
| 30 | 3.5625 | 5.4599 |
| 40 | 3.5628 | 5.4601 |
| 50 | 3.5630 | 5.4602 |
| 60 | 3.5633 | 5.4604 |
| 70 | 3.5635 | 5.4605 |
| 80 | 3.5638 | 5.4607 |
| 90 | 3.5640 | 5.4608 |
| 100 | 3.5643 | 5.4610 |
| 200 | 3.5669 | 5.4626 |
| 300 | 3.5695 | 5.4642 |
| 400 | 3.5721 | 5.4658 |
| 500 | 3.5749 | 5.4671 |
| 600 | 3.5776 | 5.4690 |
| 700 | 3.5805 | 5.4707 |
| 800 | 3.5834 | 5.4723 |
| 900 | 3.5864 | 5.4742 |
| 1000 | 3.5893 | 5.4760 |

TABLE S1: Temperature-dependent, equilibrated lattice constants of diamond (C-dia) and silicon (Si-dia) bulk, computed as a time average over 500 Born-Oppenheimer MD snapshots. Snapshot geometries are extracted randomly within the last 50 ps of the trajectories, with a minimal time interval of 10 fs. We refrain from listing the standard deviation of the individual values, as they are consistently $\lesssim 5 \cdot 10^{-5}$ Å. Further computational details, including e.g. the thermo- and barostat settings of the isothermal-isobaric (NPT) ensemble, are provided in Sec. IV of the main text.

## S2. SUPPLEMENTARY FIGURES

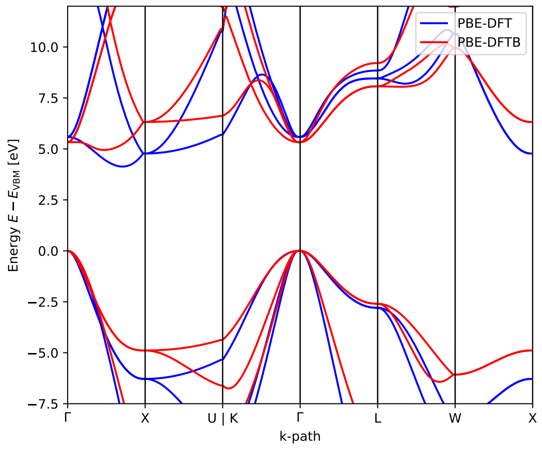


(a)

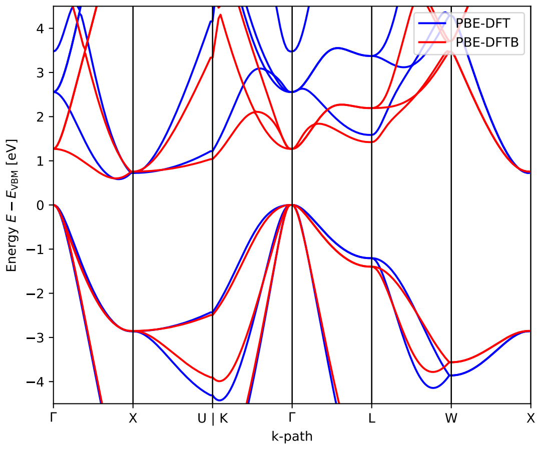


(b)

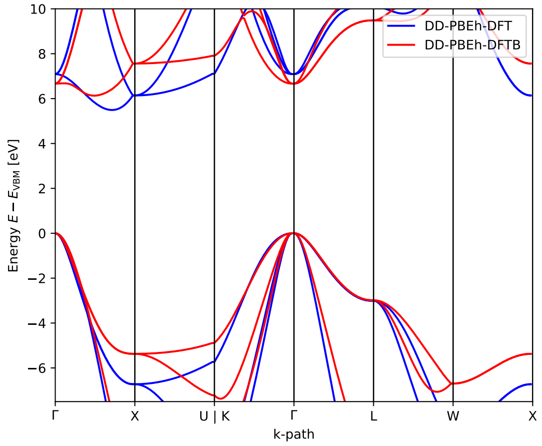


(c)

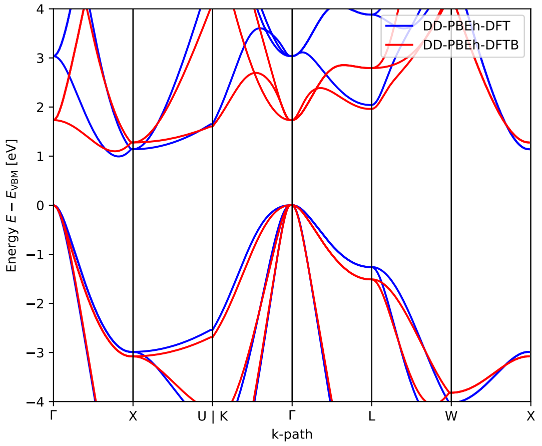


(d)

FIG. S1: Electronic bandstructures of diamond (left column) and silicon (right column) bulk, calculated on the PBE-DFTB (top row) and DD-PBEh-DFTB (bottom row) level of theory, using the parameters established in Sec. III, while DFT serves as a reference. All bandstructures have been computed at their respective experimental lattice constant [1]. Further computational details are provided in Sec. IV of the main text.

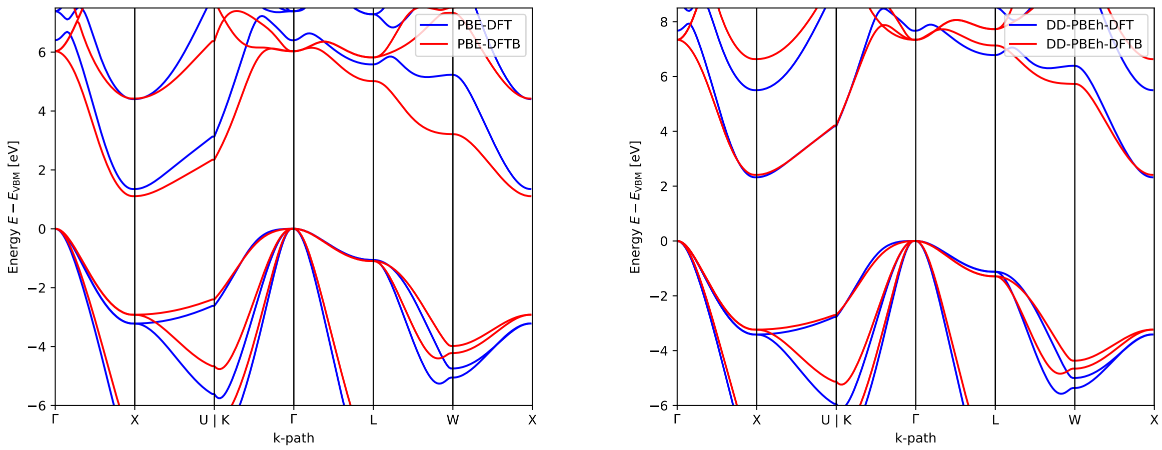


(a) PBE

(b) DD-PBEh

FIG. S2: Electronic bandstructures of zincblende structured silicon carbide (SiC-zb), computed on the PBE-DFTB (left) and DD-PBEh-DFTB (right) level of theory, using the parameters established in Sec. III of the main text, in comparison with *ab initio* DFT. All bandstructures have been computed at the experimental lattice constant $a = 4.34\,\text{Å}$ [2, 3]. Calculations based on the DD-PBEh exchange-correlation functional employ a fraction $1/\varepsilon_\infty = \alpha \approx 0.154$ [3] of global Fock-type exchange. Further computational details are provided in Sec. IV of the main text.

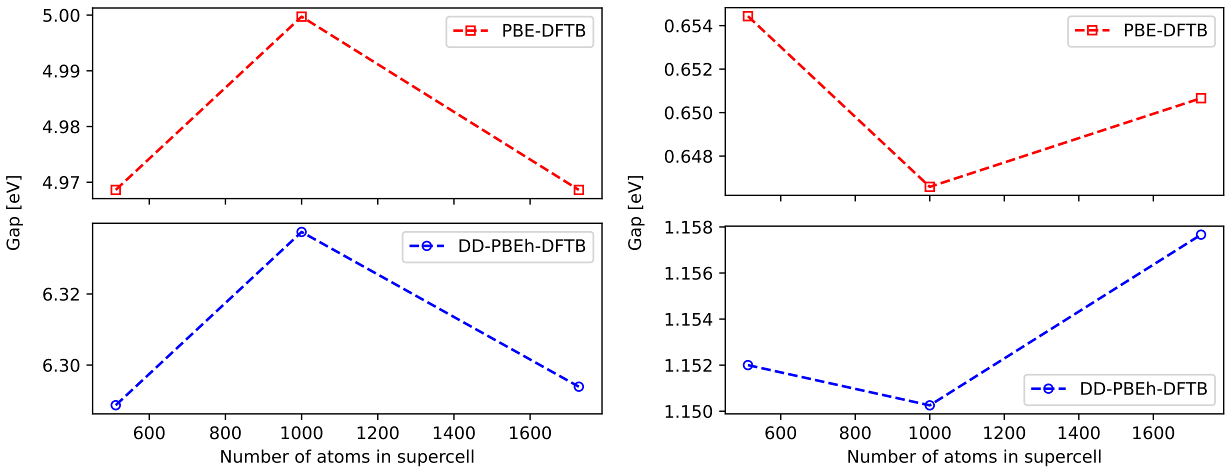


(a) diamond

(b) silicon

FIG. S3: Convergence behavior of the indirect band gap of diamond (left column) and silicon (right column) bulk w.r.t. the supercell size, computed on the PBE- and DD-PBEh-DFTB level of theory in Γ-point approximation, using the parameters established in Sec. III. The supercells are constructed from $4 \times 4 \times 4$ (512 atoms), $5 \times 5 \times 5$ (1000 atoms) and $6 \times 6 \times 6$ (1728 atoms) repetitions of the conventional unit cell, whereas the lattice constant at absolute zero is taken from Tab. S1. Further computational details are provided in Sec. IV of the main text.

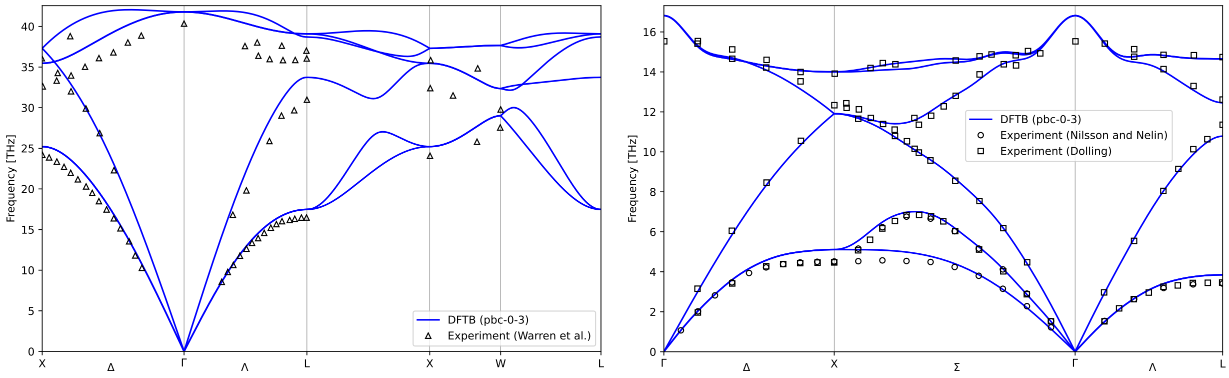


(a) diamond (b) silicon

FIG. S4: Phonon bandstructures of diamond (left) and silicon (right) bulk, calculated on the SCC-DFTB level of theory, using the pbc-0-3 [4] parameters. The results have been obtained from $8 \times 8 \times 8$ supercells build from the respective primitive unit cell (1024 atoms), as generated by the Phonopy [5, 6] code. Experimental references are taken from Ref. [7] (black triangles), Ref. [8] (black squares) and Ref. [9] (black circles).

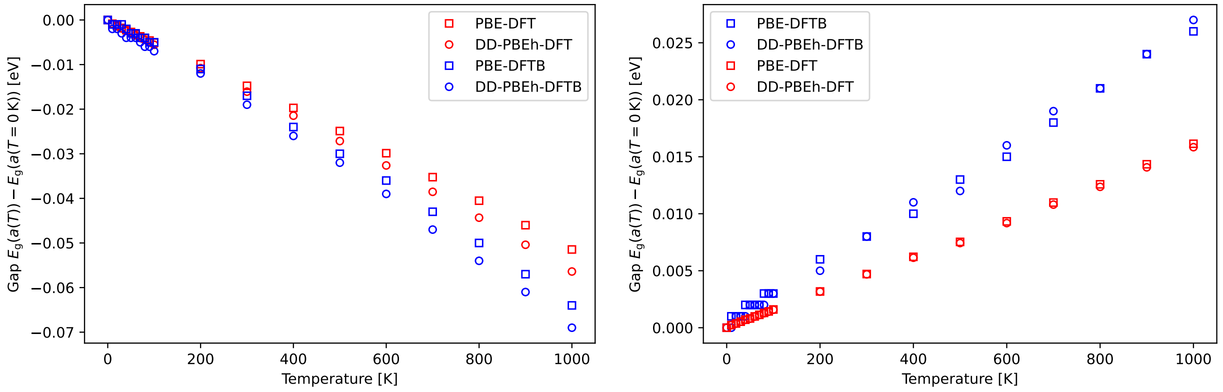


(a) diamond (b) silicon

FIG. S5: Effect of thermal lattice expansion on the indirect band gap of diamond (left) and silicon (right) bulk, calculated on the PBE-DFTB (top row) and DD-PBEh-DFTB (bottom row) level of theory, using the parameters established in Sec. III of the main text, while DFT serves as a reference. The bandstructures are computed based on a self-consistent density obtained by a $13 \times 13 \times 13$ Monkhorst-Pack [10] k-point sampling and temperature-dependent lattice parameters taken from Tab. S1.

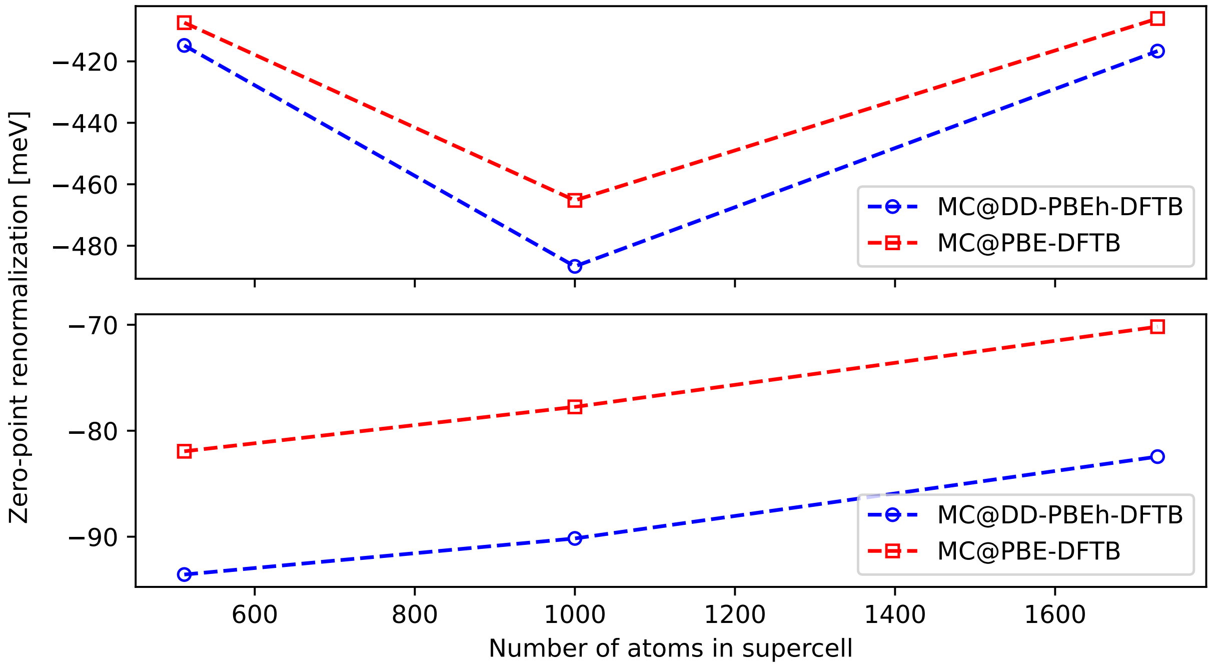


FIG. S6: Convergence behavior of the zero-point renormalization of diamond (top) and silicon (bottom) w.r.t. the supercell size, following the stochastic Monte-Carlo evaluation of Eq. (7). The supercells are constructed from $4 \times 4 \times 4$ (512 atoms), $5 \times 5 \times 5$ (1000 atoms) and $6 \times 6 \times 6$ (1728 atoms) repetitions of the conventional unit cell, whereas the lattice constant at absolute zero is taken from Tab. S1. Calculations are performed on the PBE- and DD-PBEh-DFTB level of theory, using the parameters established in Sec. III. Further computational details are provided in Sec. IV of the main text.

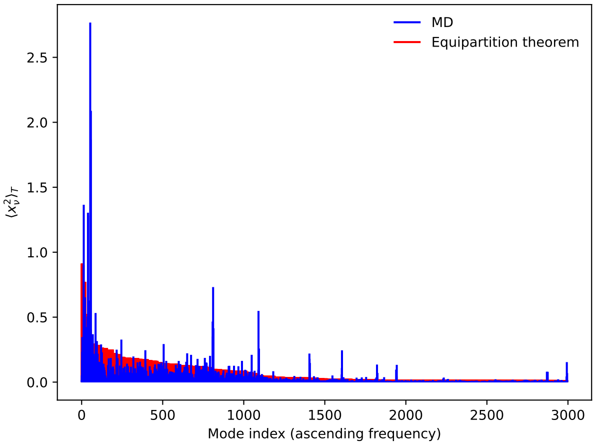


(a) $T = 50\,\mathrm{K}$

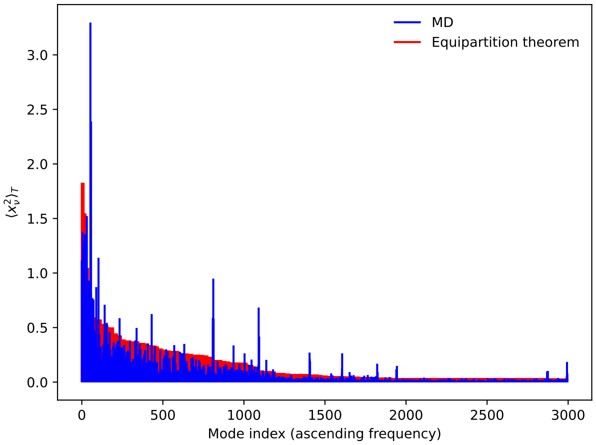


(b) $T = 100\,\mathrm{K}$

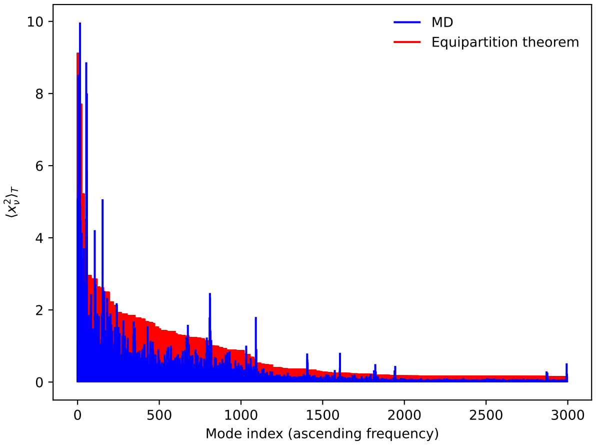


(c) $T = 500\,\mathrm{K}$

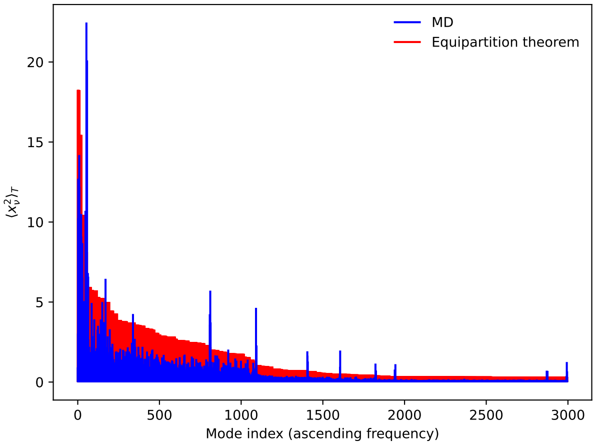


(d) $T = 1000\,\mathrm{K}$

FIG. S7: Mean square nuclear displacements $\langle x_\nu^2 \rangle_T$ at temperature $T$, determined from Eq. (12) as a time average in steps of 10 fs of the last 50 ps of each respective MD trajectory. The evaluation of Eq. (12) is based on the eigenmodes and eigenfrequencies computed in harmonic approximation, using pbc-0-3 [4] parametrized DFTB. Mean square nuclear displacements according to the equipartition principle, i.e. Eq. (15) of the main text, serve for comparison and resemble the trend of the MD.

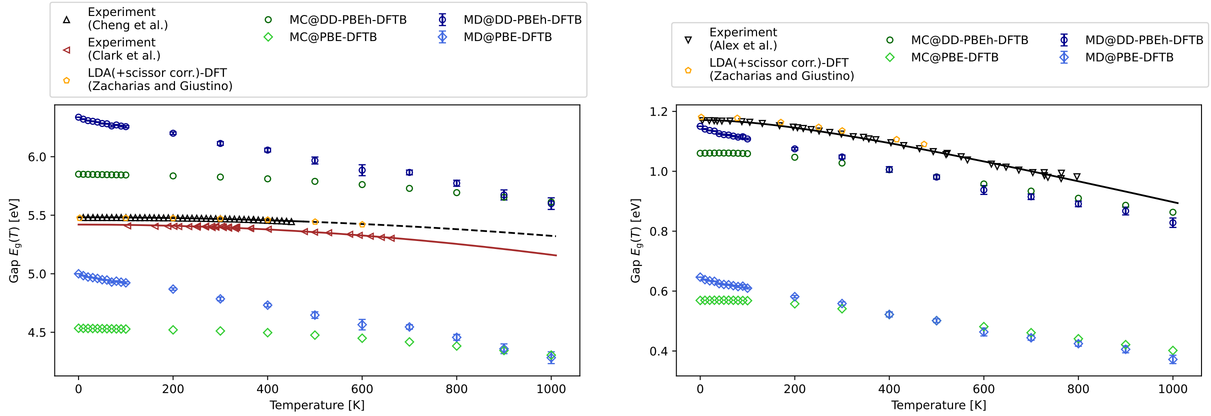


(a) diamond (b) silicon

FIG. S8: Phonon-induced band gap renormalization in absolute terms calculated on the PBE- and DD-PBEh-DFTB level of theory, using the electronic parameters established in Sec. III. Comparison is made between stochastic Monte-Carlo integration (MC) and Born-Oppenheimer molecular dynamic simulations (MD). Solid lines refer to experimental references fitted by Varshni's equation to guide the eye and provide an extrapolation (dashed segment) to higher temperatures. Further computational details are provided in Sec. IV. Experimental references are taken from Ref. [11] (black triangles up), Ref. [12] (brown triangles left) and Ref. [13] (black triangles down), in addition to the scissor-corrected LDA-DFT results of Zacharias and Giustino [14].

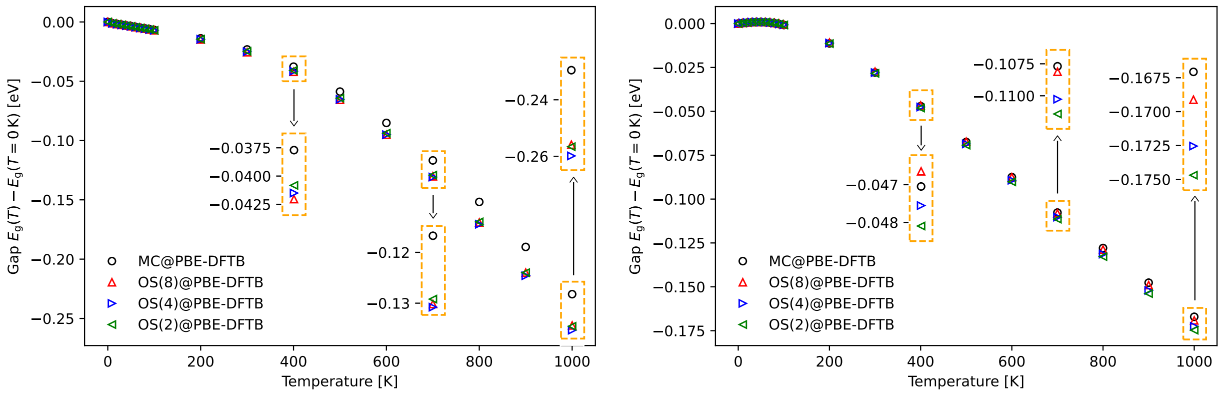


(a) diamond

(b) silicon

FIG. S9: Convergence analysis of the one-shot approach (OS) to Eq. (7), w.r.t. the number of sign configurations (indicated in round brackets). The phonon-induced band gap renormalization is calculated on the PBE-DFTB level of theory, using the parameters established in Sec. III. Further computational details are provided in Sec. IV of the main text.

---


[1] O. Madelung, *Semiconductors: data handbook*, 3rd ed. (Springer-Verlag, Berlin, Germany, 2004).

[2] L. Schimka, J. Harl, and G. Kresse, Improved hybrid functional for solids: The HSEsol functional, J. Chem. Phys. **134**, 024116 (2011).

[3] J. H. Skone, M. Govoni, and G. Galli, Self-consistent hybrid functional for condensed systems, Phys. Rev. B **89**, 195112 (2014).

[4] C. Köhler and T. Frauenheim, Molecular dynamics simulations of $CF_x$ ($x$=2,3) molecules at $Si_3N_4$ and $SiO_2$ surfaces, Surf. Sci. **600**, 453 (2006).

[5] A. Togo, First-principles Phonon Calculations with Phonopy and Phono3py, J. Phys. Soc. Jpn. **92**, 012001 (2023).

[6] A. Togo, L. Chaput, T. Tadano, and I. Tanaka, Implementation strategies in phonopy and phono3py, J. Phys. Condens. Matter **35**, 353001 (2023).

[7] J. L. Warren, J. L. Yarnell, G. Dolling, and R. A. Cowley, Lattice Dynamics of Diamond, Phys. Rev. **158**, 805 (1967).

[8] G. Dolling, *Lattice Vibrations in Crystals with the Diamond Structure* (IAEA, International Atomic Energy Agency (IAEA), 1963).

[9] G. Nilsson and G. Nelin, Study of the Homology between Silicon and Germanium by Thermal-Neutron Spectrometry, Phys. Rev. B **6**, 3777 (1972).

[10] H. J. Monkhorst and J. D. Pack, Special points for Brillouin-zone integrations, Phys. Rev. B **13**, 5188 (1976).

[11] L. Cheng, S. Zhu, X. Ouyang, and W. Zheng, Bandgap evolution of diamond, Diam. Relat. Mater. **132**, 109638 (2023).

[12] C. D. Clark, P. J. Dean, P. V. Harris, and W. C. Price, Intrinsic edge absorption in diamond, Proceedings of the Royal Society of London. Series A. Mathematical and Physical Sciences **277**, 312 (1964).

[13] V. Alex, S. Finkbeiner, and J. Weber, Temperature dependence of the indirect energy gap in crystalline silicon, J. Appl. Phys. **79**, 6943 (1996).

[14] M. Zacharias and F. Giustino, One-shot calculation of temperature-dependent optical spectra and phonon-induced band-gap renormalization, Phys. Rev. B **94**, 075125 (2016).
